# Supplementary material for: Char2char Generation with Reranking for the E2E NLG Challenge
Source: arXiv:1811.05826 source file (2018-11-04)
Supplement: Supplementary file 1 [file appendix.tex]

%\section*{Appendix: Sample predictions}

\begin{table*}
%\vspace{-85mm}
\section*{Appendix: Sample predictions}
%\centering
%\resizebox{\textwidth}{!}{%
\begin{tabular}{lll}
\hline
\textbf{Slots} &  \textbf{Type} & \textbf{Utterance}
%\multicolumn{2}{l}{}                                                                                                                                                                                                                   
\\ \hline
\hline
\multirow{2}{*}{ 3} &  MR   &  name[Blue Spice], eatType[coffee shop], area[city centre] \\ 
&  Pred &  Blue Spice is a coffee shop located in the city centre. \\ \hline

\multirow{2}{*}{ 4} &  MR   &  \begin{tabular}[c]{@{}l@{}} name[Blue Spice], eatType[coffee shop], customer rating[5 out of 5], near[Crowne \\ Plaza Hotel] \end{tabular} \\ 
& Pred &  \begin{tabular}[c]{@{}l@{}} Blue Spice is a coffee shop near Crowne Plaza Hotel with a customer rating of 5 \\ out of 5. \end{tabular} \\ \hline

\multirow{2}{*}{ 5} &  MR   &  \begin{tabular}[c]{@{}l@{}} name[The Cricketers], eatType[coffee shop], customer rating[1 out of 5], \\ familyFriendly[yes], near[Avalon] \end{tabular}\\ 
&  Pred   &  \begin{tabular}[c]{@{}l@{}} The Cricketers is a children friendly coffee shop near Avalon with a customer rating of \\ 1 out of 5. \end{tabular} \\ \hline

\multirow{2}{*}{\small 6} & \small MR   & \begin{tabular}[c]{@{}l@{}} name[Blue Spice], eatType[pub], food[Chinese], area[city centre], \\ familyFriendly[no], near[Rainbow Vegetarian Caf\'{e}] \end{tabular} \\  
&  Pred   & \begin{tabular}[c]{@{}l@{}} Blue Spice is a Chinese pub located in the city centre near Rainbow Vegetarian Caf\'{e}. \\ It is not family friendly. \end{tabular} \\ \hline

\multirow{2}{*}{ 7} & MR   & \begin{tabular}[c]{@{}l@{}} name[The Mill], eatType[pub], food[English], priceRange[high], area[riverside], \\  familyFriendly[yes], near[Raja Indian Cuisine]\end{tabular}      \\ 
&  Pred & \begin{tabular}[c]{@{}l@{}} The Mill is a children friendly English pub with a high price range near Raja Indian \\ Cuisine in riverside. \end{tabular}                                     \\ \hline

\multirow{2}{*}{8} &  MR   & \begin{tabular}[c]{@{}l@{}} name[The Cricketers], eatType[restaurant], food[Chinese], priceRange[\textsterling 20-25],  \\ customer rating[high], area[city centre], familyFriendly[no], near[All Bar One] \end{tabular} \\ 
&  Pred & \begin{tabular}[c]{@{}l@{}} The Cricketers is a restaurant providing Chinese food in the \textsterling 20-25 price range. It is \\  located in the city centre near All Bar One. It has a high customer rating and is not \\ kid friendly. \end{tabular}\\ \hline
\end{tabular}
%}
\caption{Sample predictions. For the first MR of each arity (3 to 8) in the testset, we show the prediction of our primary submission.}
\label{utterances}
\end{table*}

\begin{figure*}[]
\centering{\includegraphics[scale=.45]{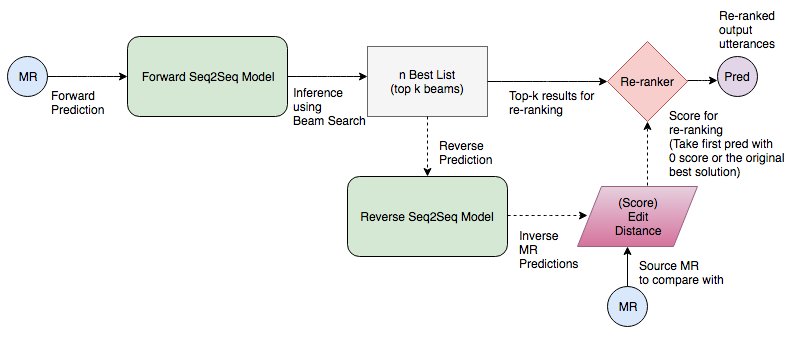}}
\caption{Illustration of the pipeline for the re-ranking approach (based on inverse reconstructions using reverse model). Apart from Forward and Reverse seq2seq models, we have a re-ranker based on the edit distance of the actual MR and the inverse reconstructed MR.}
\label{fig:ReversePipeline}
\end{figure*}
